# Supplementary material for: Joint Decision-Making in Robot Teleoperation: When are Two Heads Better Than One?
Source: arXiv:2503.15510 source file (2025-01-28)
Supplement: Supplementary file 1 [file appendix.tex]

% \clearpage
% \appendix
% \section*{APPENDIX}

% \begin{figure}
%     \centering
%     \includegraphics[width=0.9\columnwidth]{sections/figures/auroc2_hist.png}
%     \caption{Histogram of AUROC2 values over the entire set of participants.}
%     \label{fig:auroc-histogram}
% \end{figure}


% \begin{figure}
%     \centering
%     \includegraphics[width=0.9\columnwidth]{sections/figures/conf-hist.png}
%     \caption{Histogram of confidence ratings over all trials over the entire set of participants. We see that the task is suited to elicit the full range of confidence ratings from participants.}
%     \label{fig:conf-histogram}
% \end{figure}

% We conducted a pilot study with five participants to find the shortest driving time that participants felt allowed them to make a choice between the two robots. 
% Participants drove each robot for intervals of 4, 6, 8, and 10 seconds, each with 5 trials. Three fixed levels of difficulties were considered, with delay differences in the control of the two robots: 50ms - 70ms; 50ms - 90ms; 50ms - 110ms. Therefore, each participant experienced a total of 60 trials.

% At the end of the experiment, each participant was asked to identify the shortest time they found sufficient for making a decision among 4, 6, 8, or 10 seconds.
% All the participants reported that 6 seconds was the shortest time that allowed them to identify differences between two robots and make a decision.
% Further, we compared the success rate among all difficulties for the 4, 6, 8, and 10 seconds driving scenarios. The results are shown in Table~ \ref{tab:success_rate}. We find that 6 seconds also leads to our desired target success rate of 70\%.

% \begin{table}
%     \centering
%     \begin{tabular}{|c|c|}
%     \hline
%     Time (seconds) & Success rate (\%) \\
%     \hline
%     4 & 63.3 \\
%     6 & 71.2 \\
%     8 & 77.8 \\
%     10 & 91.1 \\
%     \hline
%     \end{tabular}
%     \caption{Success rate for each driving scenario}
%     \label{tab:success_rate}
% \end{table}
